# Supplementary material for: Second-Order Fine-Tuning without Pain for LLMs:A Hessian Informed Zeroth-Order Optimizer
Source: arXiv:2402.15173 source file (2025-02-18)
Supplement: Supplementary file 1 [file app_adafactor.tex]

\begin{table*}[h]
\centering
\setlength{\tabcolsep}{4pt}
\resizebox{\textwidth}{!}{
    \begin{tabular}{lcccccccccccccc}
    \toprule
    & \textbf{Model} & \textbf{Method}  & \textbf{SST-2}	& \textbf{RTE} & \textbf{CB} & \textbf{BoolQ} & \textbf{WSC} & \textbf{WIC}	& \textbf{MultiRC} & \textbf{COPA} & \textbf{ReCoRD} & \textbf{SQuAD} & \textbf{Average}\\%& \textbf{DROP} \\
    %Task type & \multicolumn{7}{c}{------------------------ classification ------------------------} & \multicolumn{2}{c}{--- multiple choice ---} & generation\\ %\multicolumn{2}{c}{--- generation ---}\\
    \midrule
    %Adam(FT) {\fontsize{8}{9.6}\selectfont (12x memory)} & {92.0} & {70.8} &	{83.9} &	{77.1}	& {63.5} &	{70.1} &71.1 &{79.0} & {74.1} &{84.9}	\\%& {31.3} \\
    &\textbf{OPT-13B} &\textbf{MeZO}	&91.4	&66.1	&67.9	&67.6	&63.5	&59.4	&60.1	&88.0	&81.7	&84.7	&73.04 \\

    &\textbf{OPT-13B} &\textbf{HiZOO}     & 92.1    &69.3	&69.6	&67.3	&63.5	&59.4	&61.3 &88.0 & 81.4 &81.9 &73.38\\

    &\textbf{OPT-13B} &\textbf{HiZOO-L}     &92.1 & 68.2  &67.9 & 66.6 &65.4 &59.4 &61.1 &88.0 &81.1 &81.9 &73.16\\

    \midrule
    %Adam(FT) {\fontsize{8}{9.6}\selectfont (12x memory)} & {92.0} & {70.8} &	{83.9} &	{77.1}	& {63.5} &	{70.1} &71.1 &{79.0} & {74.1} &{84.9}	\\%& {31.3} \\
    &\textbf{Llama3} &\textbf{MeZO}	&92.2	&74.4	&69.6	&76.7	&63.5	&57.8	&77.6	&88.0	&85.6	&86.7	&77.21\\

    &\textbf{Llama3} &\textbf{HiZOO}     & 93.5    &75.1	&69.6	&77.1	&63.5	&59.7	&78.2 &89.0 & 85.6 & 87.3 &77.85\\

    &\textbf{Llama3} &\textbf{HiZOO-L}     &94.3    &75.1	 &69.6	&76.9	&63.5	&57.7	&77.9 &89.0 & 85.6 &87.7 &77.73 \\
    
    \bottomrule
    \end{tabular}}
    \caption{
        Experiments on OPT (13B) and Llama3 (8B) with MeZO, HiZOO and HiZOO-L.
    }
    \label{tab:adafactor}
\end{table*}
