# Supplementary material for: Second-Order Fine-Tuning without Pain for LLMs:A Hessian Informed Zeroth-Order Optimizer
Source: arXiv:2402.15173 source file (2025-02-18)
Supplement: Supplementary file 2 [file app_benchmark_memory.tex]

\begin{table}[h]
\caption{Comparison of Memory and Runtime Cost as Multiples of ZO-SGD}
\centering
\begin{tabular}{lcc}
\toprule
\textbf{Optimizer} & \textbf{Memory} & \textbf{Runtime Cost} \\
\midrule
ZO-SGD & 1.0x & 1.0x \\
ZO-SGD-Cons & 1.0x & 2.49x \\
ZO-SGD-Sign & 1.0x & 1.0x \\
ZO-SGD-MMT & 1.56x & 1.0x \\
% Forward-Grad & 2.09x & 1.5x \\
% FO-SGD & 2.31x & 1.72x \\
ZO-Adam & 2.47x & 1.04x \\
% FO-Adam & 3.83x & 1.75x \\
HiZOO & 2.04x & 1.37x \\ 
HiZOO-L & 1.12x & 1.39x \\
\bottomrule
\end{tabular}
\label{app_benchmark_memory}
\end{table}
