# Supplementary material for: Second-Order Fine-Tuning without Pain for LLMs:A Hessian Informed Zeroth-Order Optimizer
Source: arXiv:2402.15173 source file (2025-02-18)
Supplement: Supplementary file 4 [file app_roberta_k16.tex]

\begin{table*}[t]
\vspace*{-2mm} 
\centering
\caption{Experiments on RoBERTa-large (350M parameters, k=16) that include zero-shot learning, linear probing (LP), full-parameter fine-tuning with Adam, MeZO and \name, and parameter-efficient fine-tuning (LoRA and prefix tuning) with Adam, MeZO and \nameo respectively. All reported numbers are averaged accuracy (standard deviation) across 5 runs. With full-parameter fine-tuning, \nameo outperforms MeZO with \textbf{3.56\%} on average on all datasets.}
    \label{app:roberta_k16}
\scalebox{0.8}{
    \begin{tabular}{lccccccc}
    \toprule
    Task Type & \multicolumn{1}{c}{\textbf{SST-2}} & \multicolumn{1}{c}{\textbf{SST-5}} & \multicolumn{1}{c}{\textbf{SNLI}}  & \multicolumn{1}{c}{\textbf{MNLI}} & \multicolumn{1}{c}{\textbf{RTE}} & \multicolumn{1}{c}{\textbf{TREC}} & \multicolumn{1}{c}{\textbf{Average}}\\
    & \multicolumn{2}{c}{------ sentiment ------} & \multicolumn{3}{c}{------ natural language inference ------} & \multicolumn{1}{c}{--- topic ---}& \multicolumn{1}{c}{--- Average ---}\\
    \midrule
    Zero-shot & 79.0  & 35.5  & 50.2  & 48.8  & 51.4  & 32.0 & 49.5\\
        LP    &  76.0 ($\pm$2.8) & 40.3 ($\pm$1.9) & 66.0 ($\pm$2.7) & 56.5 ($\pm$2.5) & 59.4 ($\pm$5.3) & 51.3 ($\pm$5.5) & 58.3\\

    \midrule
    Adam (FT)  & 91.9 ($\pm$1.8) & 47.5 ($\pm$1.9) & 77.5 ($\pm$2.6) & 70.0 ($\pm$2.3) & 66.4 ($\pm$7.2) & 85.0 ($\pm$2.5) & 73.1\\
    Adam (PEFT) & 91.4 ($\pm$1.7) & 46.7 ($\pm$1.1) & 74.9 ($\pm$4.3) & 67.7 ($\pm$1.4) & 66.1 ($\pm$3.5) & 82.7 ($\pm$4.1) & 71.6\\
    Adam (PEFT) &  91.9 ($\pm$1.0) & 47.7 ($\pm$1.1) & 77.2 ($\pm$1.3) & 66.5 ($\pm$2.5) & 66.6 ($\pm$2.0) & 85.7 ($\pm$1.3) & 72.6\\
    
    \midrule
    MeZO  & 90.5 ($\pm$1.2) & 45.5 ($\pm$2.0) & 68.5 ($\pm$3.9) & 58.7 ($\pm$2.5) & 64.0 ($\pm$3.3) & 76.9 ($\pm$2.7) & 67.4\\
    MeZO (LoRA) & 91.4 ($\pm$0.9) & 43.0 ($\pm$1.6) & 69.7 ($\pm$6.0) & 64.0 ($\pm$2.5) & 64.9 ($\pm$3.6) & 73.1 ($\pm$6.5) & 67.7\\
    MeZO (prefix) &  90.8 ($\pm$1.7) & 45.8 ($\pm$2.0) & 71.6 ($\pm$2.5) & 63.4 ($\pm$1.8) & 65.4 ($\pm$3.9) & 80.3 ($\pm$3.6) & 69.6\\
    
    \midrule
    \name  & \textbf{93.2} ($\pm$0.8) & 46.2 ($\pm$1.1) & \textbf{74.6} ($\pm$1.3) & \textbf{64.9} ($\pm$1.7) & \textbf{66.8} ($\pm$ 1.2) & 79.8 ($\pm$1.3) & 70.9\\
    \name (LoRA) & 91.2 ($\pm$0.4) & 42.9 ($\pm$0.8) & 71.1 ($\pm$1.1) & 62.1 ($\pm$1.7) & 61.4 ($\pm$2.2) & 52.2 ($\pm$3.2) & 63.5\\
    \name (prefix) & 92.3 ($\pm$1.2) & \textbf{47.2} ($\pm$1.1) & 68.8 ($\pm$1.7) & 61.6 ($\pm$1.2) & 65.4 ($\pm$1.2) & \textbf{82.0} ($\pm$2.0) & 69.6\\
    \bottomrule
    \end{tabular}}
    
\end{table*}%
